# Supplementary material for: Mechanistic study of mixed lithium halides solid state electrolytes
Source: arXiv:2511.15402 source file (2026-07-23)
Supplement: Supplementary file 1 [file SI-file.pdf]

# Supplementary Informations of Mechanistic study of mixed lithium halides solid state electrolytes

Davide Tisi,<sup>1</sup> Sergey Pozdnyakov,<sup>1</sup> and Michele Ceriotti<sup>1,\*</sup>

<sup>1</sup>*Laboratory of Computational Science and Modeling, Institut des Matériaux,  
École Polytechnique Fédérale de Lausanne, 1015 Lausanne, Switzerland*

(Dated: November 14, 2025)

---

\* michele.ceriotti@epfl.ch

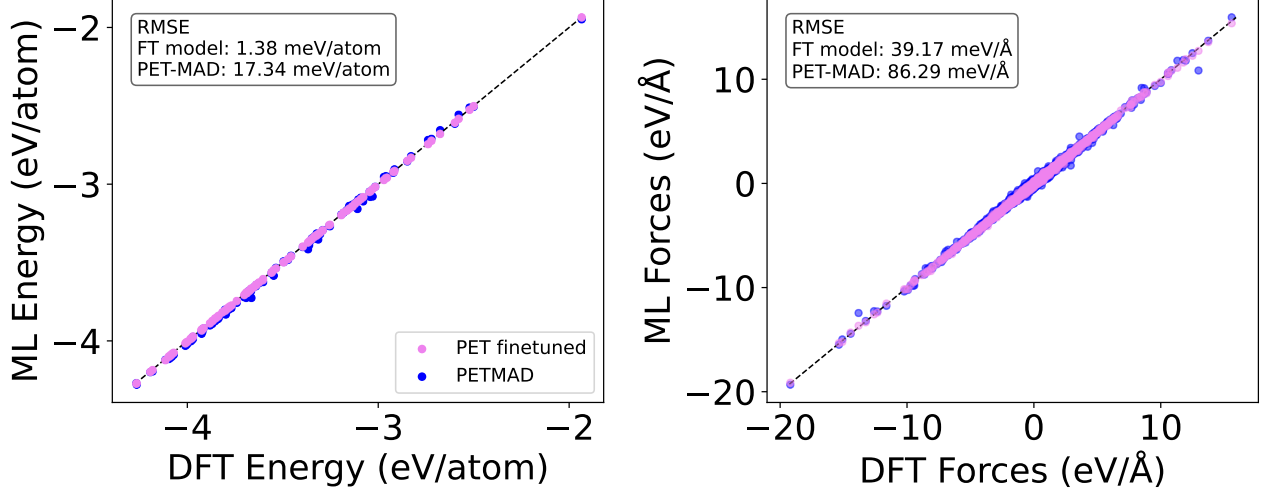

FIG. S1. Parity plot of the energy (left panel) and atomic forces (right panel) for the PET-MAD universal potential and PET-fine-tuned model.

### I. PARITY PLOT

Fig. S1 shows the parity plot for energy and forces of the PET-MAD universal potential (blue) and the finetuned model (violet) computed for a test set. The figure also shows the root-mean-square-errors (RMSE) for both energies and forces of both models. The RMSE is computed using these definitions:

$$RMSE_E = \sqrt{\frac{\sum_t (E_t^{ML} - E_t^{DFT})^2}{N_{set}}} \quad (S1)$$

$$RMSE_F = \sqrt{\frac{\sum_t \sum_j \sum_{\alpha \in x,y,z} (F_{tj\alpha}^{ML} - F_{tj\alpha}^{DFT})^2}{3N_{atoms}}} \quad (S2)$$

where  $E_t^{ML}$  and  $E_t^{DFT}$  are the energy of snapshot  $t$  predicted by the ML model and by the DFT reference, respectively. The sum of  $t$  runs over all the  $N_{set}$  snapshots in the test set.  $F_{tj\alpha}^{ML}$  and  $F_{tj\alpha}^{DFT}$  represent the prediction of the  $\alpha$  component of the force acting on atom  $j$  in the snapshot  $t$ .  $N_{atoms}$  represents the total number of atoms in all the structures in the test set.

### II. SIZE SCALING

Fig. S2 shows conductivity as a function of the size of the system for the system of pure Br and Cl in both crystal structures. The vertical dashed lines represent the size of 960 atoms, used in the main results of this work. At that size the result is completely converged.

### III. MC STABILITY

Fig. S3 shows the evolution of the acceptance rate of Monte Carlo (MC) swaps during the simulation of  $\text{LiYBr}_{6(1-x)}\text{Cl}_{6x}$  in the both phases at all the different compositions. After an initial thermalization period, the system reaches a stable number of accepted swaps, indicating equilibration. On average 12% of swaps-per-step are accepted.

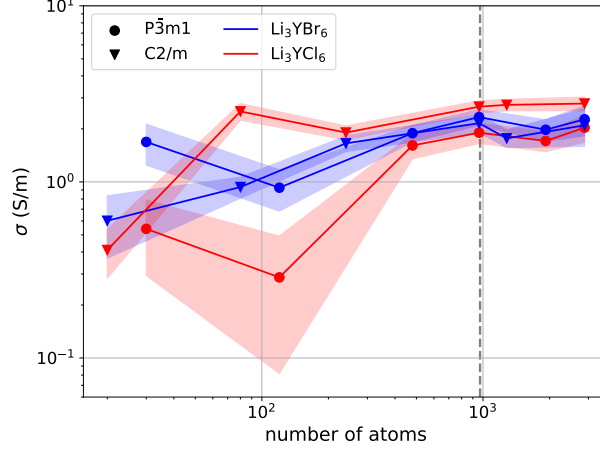

FIG. S2. Size scaling of the conductivity for different structures and lattice

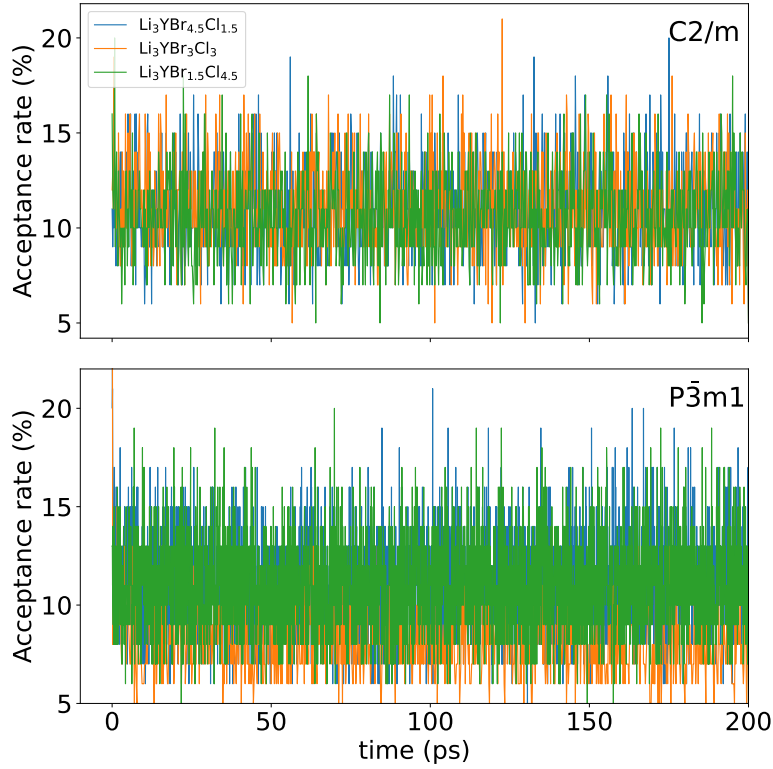

FIG. S3. Acceptance rate during the Monte Carlo simulations of  $\text{Li}_3\text{YBr}_{6(1-x)}\text{Cl}_{6x}$  in the C2/m (upper panel) and  $\text{P}\bar{3}\text{m}1$  (lower panel) phase at all the different compositions.

#### IV. RADIAL DISTRIBUTION FUNCTION OF STRUCTURE OF DIFFERENT MC SIMULATION

Fig. S4 shows the partial radial distribution functions (RDFs) for the 4 configurations of  $\text{Li}_3\text{YBr}_3\text{Cl}_3$  in the  $\text{P}\bar{3}\text{m}1$  phase extracted from the MC simulation. The top panel shows the partial RDFs of the halogen atoms, while the lower panel shows the RDF between the Y and the halogen atoms. In all cases the RDFs for different snapshot are perfectly on top of each other, showing that different snapshots extracted from the MC simulations have the same structure.

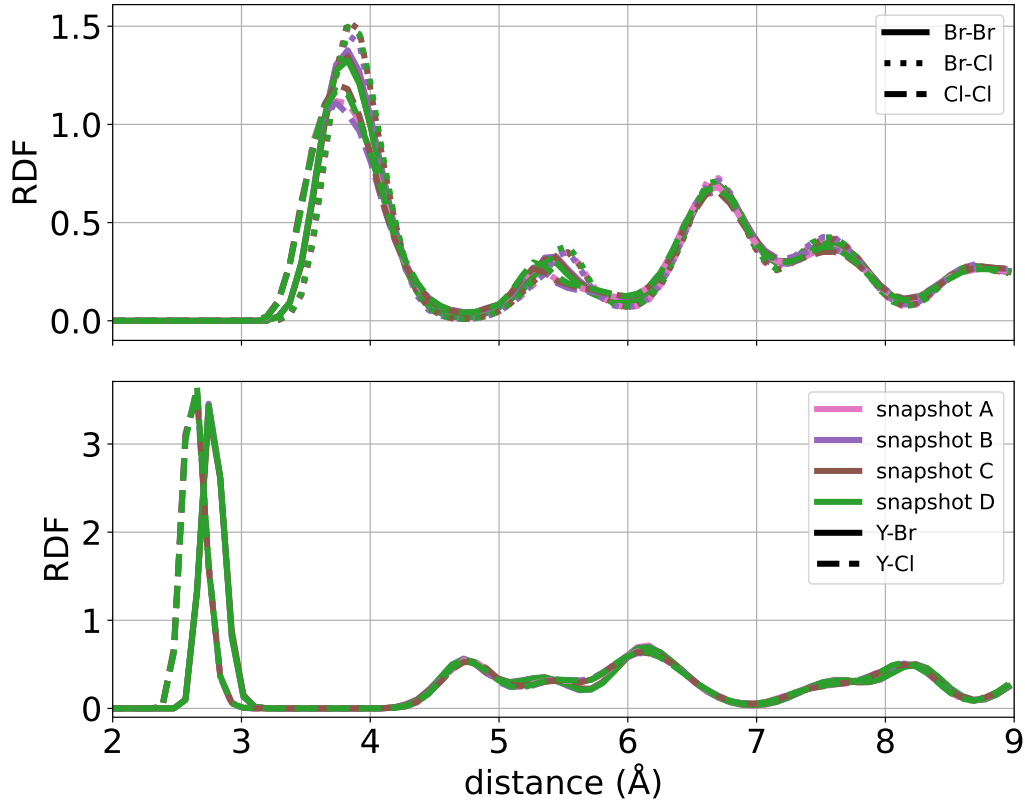

FIG. S4. Radial distribution functions (RDF) of 4 configuration of  $\text{Li}_3\text{YBr}_3\text{Cl}_3$  in the  $P\bar{3}m1$  phase. Upper panel contains the RDF between the different halogen atoms: Br-Br (continuous), Br-Cl (dotted), Cl-Cl (dashed). Lower panel contains the RDF between the Y atoms and the halogens: Y-Br (continuous), Y-Cl (dashed). These are extracted from the final 50 ps of 2 ns long NPT simulations.

## V. EFFECTS OF ALLOYING ON THE CONDUCTIVITY

In the main text we show the effects of alloying on the conductivity showing, in the cases of mixed composition, the average conductivity of different snapshot at the same Br-Cl ratio. Fig. S5 is the equivalent of Fig. 5 in the main text, where for the mixed compositions each point correspond to the  $\sigma$  extracted from a simulation done with one of the structures selected from the MC simulation.

- 
- [1] Zhantao Liu, Shuan Ma, Jue Liu, Shan Xiong, Yifan Ma, and Hailong Chen, “High Ionic Conductivity Achieved in  $\text{Li}_3\text{Y}(\text{Br}_3\text{Cl}_3)$  Mixed Halide Solid Electrolyte via Promoted Diffusion Pathways and Enhanced Grain Boundary,” *ACS Energy Letters* **6**, 298–304 (2021).
  - [2] Tetsuya Asano, Akihiro Sakai, Satoru Ouchi, Masashi Sakaida, Akinobu Miyazaki, and Shinya Hasegawa, “Solid Halide Electrolytes with High Lithium-Ion Conductivity for Application in 4 V Class Bulk-Type All-Solid-State Batteries,” *Advanced Materials* **30**, 1–7 (2018).
  - [3] Eveline van der Maas, Wenxuan Zhao, Zhu Cheng, Theodosios Famprikis, Michel Thijs, Steven R. Parnell, Swapna Ganapathy, and Marnix Wagemaker, “Investigation of structure, ionic conductivity, and electrochemical stability of halogen substitution in solid-state ion conductor  $\text{Li}_3\text{YBr}_3\text{Cl}_{6-x}$ ,” *The Journal of Physical Chemistry C* **127**, 125–132 (2023).

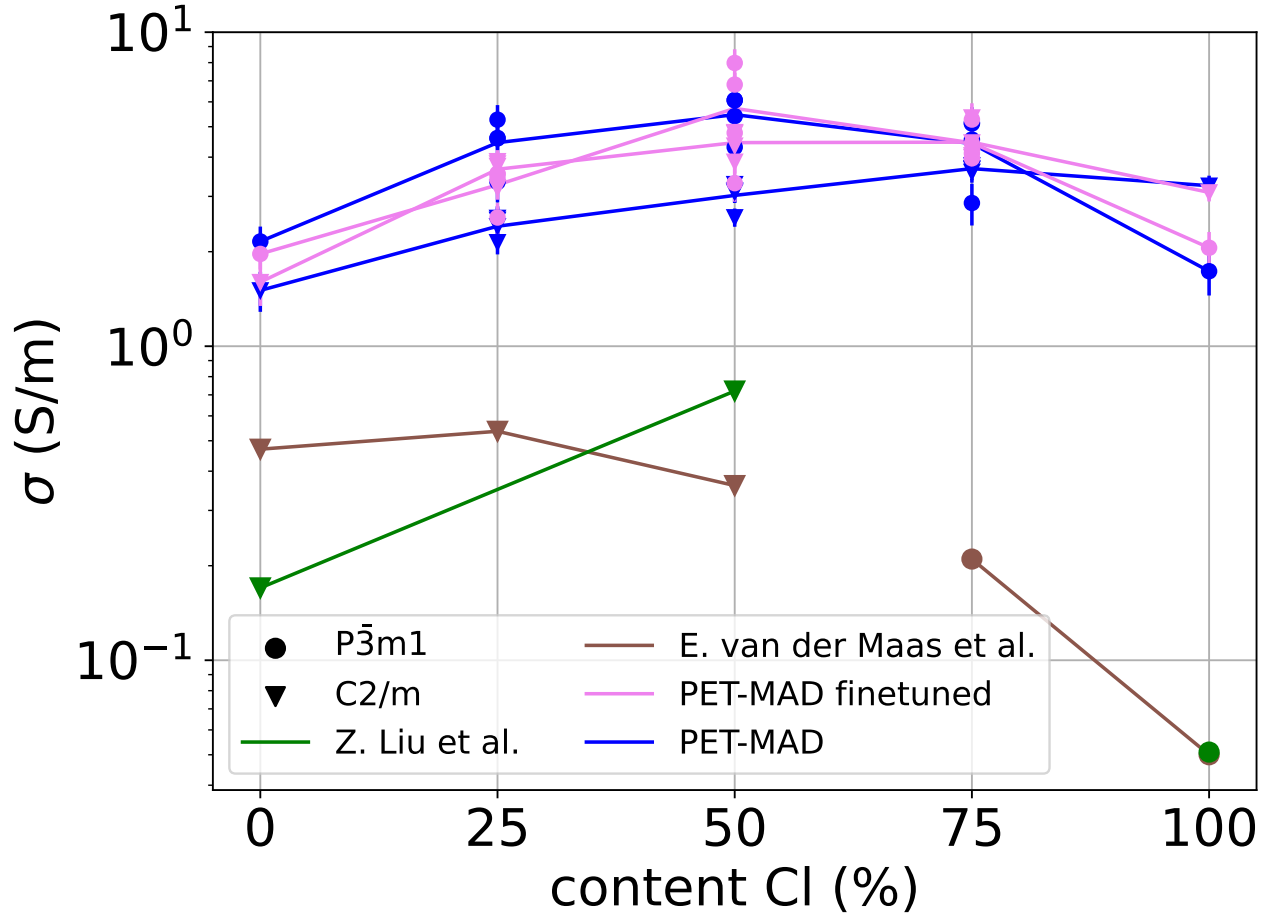

FIG. S5. Ionic conductivity ( $\sigma$ ) of  $\text{Li}_3\text{YBr}_{6(1-x)}\text{Cl}_6x$ , with  $x \in [0, 1]$ , as a function of percentage of Cl content, computed via the PET-MAD universal potential (blue) and a PET model fine-tuned (pink line) on a specific dataset. Each point is the result of a calculation on a particular structure extracted from the MC procedure and the lines connects the average values as presented in Fig. 5 of the main text. Results are compared with experimental results reported in Ref. [1, 2] (green) and Ref. [3] (brown).
